# Supplementary material for: AdapterBias: Parameter-efficient Token-dependent Representation Shift for Adapters in NLP Tasks
Source: arXiv:2205.00305 source file (2023-01-30)
Supplement: Supplementary file 1 [file param.tex]

\begin{table}[]
\begin{tabular}{l|l}
\hline
\multicolumn{1}{c|}{} & Params \\ \hline
$L_\alpha$              & 3073   \\ \hline
\textit{v}                & 768    \\ \hline
\end{tabular}
\caption{
The parameter of our AdapterBias. 
}
\end{table}
